# Supplementary material for: Universality of AdaGrad Stepsizes for Stochastic Optimization: Inexact Oracle, Acceleration and Variance Reduction
Source: arXiv:2406.06398 source file (2024-06-10)
Supplement: Supplementary file 1 [file UniversalFastSgd.tex]

\subsection{Universal Fast SGD}

\begin{lemma}[Stochastic Triangle Step]
  \label{th:StochasticTriangleStep}
  Consider problem~\eqref{eq:Problem} under \cref{as:ApproximateSmoothness}.
  Let $\hat{g}$ be an unbiased oracle for $\bar{g}$,
  let $x, v \in \EffectiveDomain \psi$ be points and
  $M, A \geq 0$, $a > 0$ be coefficients.
  Further, for $A_+ \DefinedEqual A + a$, let
  \[
    y = \frac{A x + a v}{A_+},
    \quad
    \hat{g}_y \EqualRandom \hat{g}(y),
    \quad
    \hat{v}_+ = \ProximalMap_{\psi}(v, \hat{g}_y, M / a),
    \quad
    \hat{x}_+ = \frac{A x + a \hat{v}_+}{A_+}.
  \]
  Denote
  $
    \hat{\Delta}(M)
    \DefinedEqual
    \beta_{f, \bar{f}, \bar{g}}(y, \hat{x}_+)
    +
    \InnerProduct{\bar{g}(y) - \hat{g}_y}{\hat{x}_+ - y}
    -
    \frac{M A_+}{2 a^2} \Norm{\hat{x}_+ - y}^2
  $.
  Then,
  \begin{multline*}
    \Expectation\Bigl[
      A_+ [F(\hat{x}_+) - F^*] + \frac{M}{2} \Norm{\hat{v}_+ - x^*}^2
    \Bigr]
    +
    A \beta_{f, \bar{f}, \bar{g}}(y, x)
    +
    a \beta_{f, \bar{f}, \bar{g}}(y, x^*)
    \\
    \leq
    A [F(x) - F^*]
    +
    \frac{M}{2} \Norm{v - x^*}^2
    +
    A_+ \Expectation[\hat{\Delta}(M)].
  \end{multline*}
  If further \cref{as:BoundedFeasibleSet} is satisfied, and $\hat{M}_+ \geq M$
  is a random coefficient (possibly dependent on~$\hat{g}_y$),
  then we also have
  \begin{multline*}
    \Expectation\Bigl[
      A_+ [F(\hat{x}_+) - F^*] + \frac{\hat{M}_+}{2} \Norm{\hat{v}_+ - x^*}^2
    \Bigr]
    +
    A \beta_{f, \bar{f}, \bar{g}}(y, x)
    +
    a \beta_{f, \bar{f}, \bar{g}}(y, x^*)
    \\
    \leq
    A [F(x) - F^*]
    +
    \frac{M}{2} \Norm{v - x^*}^2
    +
    \Expectation[A_+ \hat{\Delta}(\hat{M}_+) + (\hat{M}_+ - M) D^2],
  \end{multline*}
\end{lemma}

\begin{proof}
  Denoting
  $
    \theta
    \DefinedEqual
    A \beta_{f, \bar{f}, \bar{g}}(y, x)
    +
    a \beta_{f, \bar{f}, \bar{g}}(y, x^*)
  $
  and using the fact that $\Expectation[\hat{g}_y] = \bar{g}(y)$,
  we can rewrite
  \begin{align*}
    \hspace{2em}&\hspace{-2em}
    A F(x) + a F(x^*) + \frac{M}{2} \Norm{v - x^*}^2
    \\
    &=
    \begin{multlined}[t]
      A [
        \bar{f}(y)
        +
        \InnerProduct{\bar{g}(y)}{x - y}
        +
        \beta_{f, \bar{f}, \bar{g}}(y, x)
        +
        \psi(x)
      ]
      \\
      +
      a [
        \bar{f}(y)
        +
        \InnerProduct{\bar{g}(y)}{x^* - y}
        +
        \beta_{f, \bar{f}, \bar{g}}(y, x^*)
        +
        \psi(x^*)
      ]
      +
      \frac{M}{2} \Norm{v - x^*}^2
    \end{multlined}
    \\
    &=
    A_+ \bar{f}(y)
    +
    \InnerProduct{\bar{g}(y)}{A x + a x^* - A_+ y}
    +
    A \psi(x) + a \psi(x^*)
    +
    \frac{M}{2} \Norm{v - x^*}^2
    +
    \theta
    \\
    &=
    \Expectation\Bigl[
      A_+ \bar{f}(y)
      +
      \InnerProduct{\hat{g}_y}{A x + a x^* - A_+ y}
      +
      A \psi(x) + a \psi(x^*)
      +
      \frac{M}{2} \Norm{v - x^*}^2
    \Bigr]
    +
    \theta.
  \end{align*}
  Further, by the definition of~$\hat{v}_+$ and
  \cref{th:OptimalityConditionForProximalStep},
  \[
    \InnerProduct{\hat{g}_y}{x^* - \hat{v}_+} + \psi(x^*)
    +
    \frac{M}{2 a} \Norm{v - x^*}^2
    \geq
    \psi(\hat{v}_+)
    +
    \frac{M}{2 a} \Norm{v - \hat{v}_+}^2
    +
    \frac{M}{2 a} \Norm{\hat{v}_+ - x^*}^2.
  \]
  This means that
  \begin{align*}
    &
    A_+ \bar{f}(y)
    +
    \InnerProduct{\hat{g}_y}{A x + a x^* - A_+ y}
    +
    A \psi(x) + a \psi(x^*)
    +
    \frac{M}{2} \Norm{v - x^*}^2
    \\
    &\geq
    A_+ \bar{f}(y)
    +
    \InnerProduct{\hat{g}_y}{A x + a \hat{v}_+ - A_+ y}
    +
    A \psi(x) + a \psi(\hat{v}_+)
    +
    \frac{M}{2} \Norm{v - \hat{v}_+}^2
    +
    \frac{M}{2} \Norm{\hat{v}_+ - x^*}^2
    \\
    &\geq
    A_+ [\bar{f}(y) + \InnerProduct{\hat{g}_y}{\hat{x}_+ - y} + \psi(\hat{x}_+)]
    +
    \frac{M}{2} \Norm{v - \hat{v}_+}^2
    +
    \frac{M}{2} \Norm{\hat{v}_+ - x^*}^2
    \\
    &=
    A_+ F(\hat{x}_+)
    +
    \frac{M}{2} \Norm{\hat{v}_+ - x^*}^2
    -
    A_+ \hat{\Delta}(M),
  \end{align*}
  where the second inequality is due to the definition of~$\hat{x}_+$
  and the convexity of~$\psi$, and
  \begin{align*}
    \hat{\Delta}(M)
    &\DefinedEqual
    f(\hat{x}_+) - \bar{f}(y) - \InnerProduct{\hat{g}_y}{\hat{x}_+ - y}
    -
    \frac{M}{2 A_+} \Norm{v - \hat{v}_+}^2
    \\
    &=
    \beta_{f, \bar{f}, \bar{g}}(y, \hat{x}_+)
    +
    \InnerProduct{\bar{g}(y) - \hat{g}_y}{\hat{x}_+ - y}
    -
    \frac{M A_+}{2 a^2} \Norm{\hat{x}_+ - y}^2
  \end{align*}
  since $\hat{x}_+ - y = \frac{a}{A_+} (\hat{v}_+ - v)$
  (by the definitions of~$y$ and~$\hat{x}_+$).
  Substituting the above inequality into the first display and rearranging, we
  get the first of the claimed inequalities.

  To prove the second one, we simply add to both sides of the already proved
  first inequality the expected value of
  \[
    \frac{\hat{M}_+ - M}{2} \Norm{\hat{v}_+ - x^*}^2
    +
    A_+ [\hat{\Delta}(M) - \hat{\Delta}(\hat{M}_+)]
    =
    \frac{\hat{M}_+ - M}{2} \Bigl(
      \Norm{\hat{v}_+ - x^*}^2
      +
      \frac{A_+^2}{a^2} \Norm{\hat{x}_+ - y}^2
    \Bigr)
  \]
  and then bound, using the fact that
  $\hat{x}_+ - y = \frac{a}{A_+} (\hat{v}_+ - v)$
  together with our \cref{as:BoundedFeasibleSet},
  \[
    \Norm{\hat{v}_+ - x^*}^2 + \frac{A_+^2}{a^2} \Norm{\hat{x}_+ - y}^2
    =
    \Norm{\hat{v}_+ - x^*}^2 + \Norm{\hat{v}_+ - v}^2
    \leq
    2 D^2.
    \qedhere
  \]
\end{proof}

\begin{lemma}[Universal Stochastic Triangle Step]
  \label{th:UniversalTriangleStep}
  Consider problem~\eqref{eq:Problem} under
  \cref{as:BoundedFeasibleSet,as:ApproximateSmoothness},
  and let $\hat{g}$ be an unbiased oracle for $\bar{g}$.
  Let $x, v \in \EffectiveDomain \psi$ be points, $M, A \geq 0$,
  $a > 0$ be coefficients.
  Further, for $A_+ \DefinedEqual A + a$, let
  \begin{gather*}
    y = \frac{A x + a v}{A_+},
    \quad
    \hat{g}_y \EqualRandom \hat{g}(y),
    \quad
    \hat{v}_+ = \ProximalMap_{\psi}(v, \hat{g}_y, M / a),
    \quad
    \hat{x}_+ = \frac{A x + a \hat{v}_+}{A_+},
    \\
    \hat{g}_{x_+} \EqualRandom \hat{g}(\hat{x}_+),
    \quad
    \hat{M}_+
    =
    \frac{a^2}{A_+}
    M_+\Bigl(
      \frac{A_+}{a^2} M, \frac{a^2}{A_+^2} D^2, y, \hat{x}_+,
      \hat{g}_y, \hat{g}_{x_+}
    \Bigr).
  \end{gather*}
  Then, for any $\bar{M} > c_2 L_f \frac{a^2}{A_+}$, it holds that
  \begin{multline*}
    \Expectation\Bigl[
      A_+ [F(\hat{x}_+) - F^*]
      +
      \frac{\hat{M}_+}{2} \Norm{\hat{v}_+ - x^*}^2
      +
      A_+ \beta_{f, \bar{f}, \bar{g}}(\hat{x}_+, y)
    \Bigr]
    +
    A \beta_{f, \bar{f}, \bar{g}}(y, x)
    +
    a \beta_{f, \bar{f}, \bar{g}}(y, x^*)
    \\
    \leq
    A [F(x) - F^*]
    +
    \frac{M}{2} \Norm{v - x^*}^2
    +
    \frac{c_1 a^2}{\bar{M} - c_2 L_f \frac{a^2}{A_+}}
    \Expectation[\Variance_{\hat{g}}(\hat{x}_+) + \Variance_{\hat{g}}(y)]
    \\
    +
    c_3 A_+ \delta_f
    +
    c_4 \Expectation\bigl\{
      \PositivePart{\min\Set{\hat{M}_+, \bar{M}} - M} D^2
    \bigr\}.
  \end{multline*}
\end{lemma}

\begin{proof}
  According to \cref{th:StochasticTriangleStep}
  (together with the fact that $\hat{M}_+ \geq M$ which is guaranteed by the
    requirement on the stepsize update rule), we have
  \begin{multline*}
    \Expectation\Bigl[
      A_+ [F(\hat{x}_+) - F^*]
      +
      \frac{\hat{M}_+}{2} \Norm{\hat{v}_+ - x^*}^2
    \Bigr]
    +
    A \beta_{f, \bar{f}, \bar{g}}(y, x)
    +
    a \beta_{f, \bar{f}, \bar{g}}(y, x^*)
    \\
    \leq
    A [F(x) - F^*]
    +
    \frac{M}{2} \Norm{v - x^*}^2
    +
    \Expectation\bigl[
      A_+ \hat{\Delta}(\hat{M}_+) + (\hat{M}_+ - M) D^2
    \bigr],
  \end{multline*}
  where
  $
    \hat{\Delta}(\hat{M}_+)
    \DefinedEqual
    \beta_{f, \bar{f}, \bar{g}}(y, \hat{x}_+)
    +
    \InnerProduct{\bar{g}(y) - \hat{g}_y}{\hat{x}_+ - y}
    -
    \frac{\hat{M}_+ A_+}{2 a^2} \Norm{\hat{x}_+ - y}^2
  $.
  Further, according to the main
  requirement~\eqref{eq:RequirementOnStepsizeUpdateRule} on the stepsize update
  rule (applied in the variables $M' \DefinedEqual \frac{A_+}{a^2} M$,
    $\Omega \DefinedEqual \frac{a^2}{A_+^2} D^2$,
    $\hat{M}_+' \DefinedEqual \frac{A_+}{a^2} \hat{M}_+$,
    $\bar{M}' \DefinedEqual \frac{A_+}{a^2} \bar{M}$
    for which we have $M' \Omega = M \frac{D^2}{A_+}$,
    $\hat{M}_+' \Omega = \hat{M}_+ \frac{D^2}{A_+}$,
    $\bar{M}' \Omega = \bar{M} \frac{D^2}{A_+}$),
  it holds that
  \begin{multline*}
    \Expectation\Bigl[
      \hat{\Delta}(\hat{M}_+)
      +
      (\hat{M}_+ - M) \frac{D^2}{A_+}
      +
      \beta_{f, \bar{f}, \bar{g}}(\hat{x}_+, y)
    \Bigr]
    \\
    \leq
    \frac{c_1}{\frac{A_+}{a^2} \bar{M} - c_2 L_f}
    \Expectation[\Variance_{\hat{g}}(\hat{x}_+) + \Variance_{\hat{g}}(y)]
    +
    c_3 \delta_f
    +
    c_4 \Expectation\Bigl\{
      \PositivePart{\min\Set{\hat{M}_+, \bar{M}} - M} \frac{D^2}{A_+}
    \Bigr\},
  \end{multline*}
  where $\bar{M} > c_2 L_f \frac{a^2}{A_+}$ is an arbitrary constant.
  Multiplying both sides of the above display by~$A_+$ and adding the result
  to the first display, we obtain the claim.
\end{proof}

\begin{lemma}[Universal Fast SGD: General Guarantee]
  \label{th:UniversalFastSgd-GeneralGuarantee}
  Consider \cref{alg:UniversalFastSgd} applied to problem~\eqref{eq:Problem}
  under \cref{as:BoundedFeasibleSet,as:ApproximateSmoothness}.
  Then, for any $k \geq 1$ and any $\bar{M} > c_2 L_f$,
  it holds that
  \begin{multline*}
    \Expectation\Bigl[
      A_k [F(x_k) - F^*]
      +
      \sum_{i = 0}^{k - 1} [
        A_{i + 1} \beta_{f, \bar{f}, \bar{g}}(x_{i + 1}, y_i)
        +
        a_{i + 1} \beta_{f, \bar{f}, \bar{g}}(y_i, x^*)
      ]
    \Bigr]
    \\
    \leq
    c_4 \bar{M} D^2
    +
    \frac{c_1}{\bar{M} - c_2 L_f}
    \sum_{i = 0}^{k - 1} a_{i + 1}^2 \Expectation[
      \Variance_{\hat{g}}(x_{i + 1}) + \Variance_{\hat{g}}(y_i)
    ]
    +
    c_3 \delta_f \sum_{i = 1}^k A_i,
  \end{multline*}
  where $a_k = \frac{1}{2} k$, $A_k = \frac{1}{4} k (k + 1)$,
  $\sum_{i = 1}^k a_i^2 = \frac{1}{24} k (k + 1) (2 k + 1)$,
  $\sum_{i = 1}^k A_i = \frac{1}{12} k (k + 1) (k + 2)$
  for each $k \geq 1$.
\end{lemma}

\begin{proof}
  Each iteration~$k$ of the algorithm, when conditioned on $(x_k, v_k)$,
  follows the construction from \cref{th:UniversalTriangleStep}
  (with $x = x_k$, $v = v_k$, $M = M_k$, $A = A_k$, $a = a_{k + 1}$,
    $A_+ = A_{k + 1}$, $y = y_k$, $\hat{g}_y = g_{y_k}$,
    $\hat{v}_+ = v_{k + 1}$, $\hat{x}_+ = x_{k + 1}$,
    $\hat{g}_{x_+} = g_{x_{k + 1}}$, $\hat{M}_+ = M_{k + 1}$),
  where $A_k$ and $a_k$ are the following coefficients:
  $a_k = \frac{1}{2} k$, $A_k = \sum_{i = 1}^k a_i = \frac{1}{4} k (k + 1)$.
  Applying \cref{th:UniversalTriangleStep} (dropping the nonnegative
    $\beta_{f, \bar{f}, \bar{g}}(y, x)$ term) and passing to full expectations,
  we therefore obtain, for each $k \geq 0$,
  \begin{multline*}
    \Expectation\Bigl[
      A_{k + 1} [F(x_{k + 1}) - F^*]
      +
      \frac{M_{k + 1}}{2} \Norm{v_{k + 1} - x^*}^2
      +
      A_{k + 1} \beta_{f, \bar{f}, \bar{g}}(x_{k + 1}, y_k)
      +
      a_{k + 1} \beta_{f, \bar{f}, \bar{g}}(y_k, x^*)
    \Bigr]
    \\
    \leq
    \Expectation\Bigl[
      A_k [F(x_k) - F^*]
      +
      \frac{M_k}{2} \Norm{v_k - x^*}^2
      +
      \frac{c_1 a_{k + 1}^2}{\bar{M} - c_2 L_f \frac{a_{k + 1}^2}{A_{k + 1}}}
      [\Variance_{\hat{g}}(x_{k + 1}) + \Variance_{\hat{g}}(y_k)]
    \Bigr]
    \\
    +
    c_3 A_{k + 1} \delta_f
    +
    c_4 \Expectation\bigl\{
      \PositivePart{\min\Set{M_{k + 1}, \bar{M}} - M_k} D^2
    \bigr\},
  \end{multline*}
  where $\bar{M}$ is an arbitrary constant such that
  $\bar{M} > c_2 L_f \frac{a_{k + 1}^2}{A_{k + 1}}$.
  Note however that, for our sequences $a_k$ and $A_k$, we have
  $
    \frac{a_k^2}{A_k}
    =
    \frac{\frac{1}{4} k^2}{\frac{1}{4} k (k + 1)}
    =
    \frac{k}{k + 1}
    \leq
    1
  $.
  Therefore, we can replace
  $
    \frac{
      c_1 a_{k + 1}^2
    }{
      \bar{M} - c_2 L_f \frac{a_{k + 1}^2}{A_{k + 1}}
    }
  $
  in the above display with $\frac{c_1 a_{k + 1}^2}{\bar{M} - c_2 L_f}$
  under the requirement that $\bar{M} > c_2 L_f$.
  Doing this and then telescoping the above inequalities
  (applying \cref{th:TelescopingDifferencesWithMin}),
  and using the fact that $M_0 = A_0 = 0$, we get the claimed inequality.

  It remains to do some standard computations to see that
  $
    \sum_{i = 1}^k a_i^2
    \equiv
    \frac{1}{4} \sum_{i = 1}^k i^2
    =
    \frac{1}{24} k (k + 1) (2 k + 1)
  $
  and
  $
    \sum_{i = 1}^k A_i
    \equiv
    \frac{1}{4} \sum_{i = 1}^k i (i + 1)
    =
    \frac{1}{4} (\frac{1}{6} k (k + 1) (2 k + 1) + \frac{1}{2} k (k + 1))
    =
    \frac{1}{12} k (k + 1) (k + 2)
  $.
\end{proof}

\thComplexityOfUniversalFastSgd*

\begin{proof}
  \label{th:UniversalFastSgd:Proof}
  Let $k \geq 1$ be arbitrary and
  $F_k \DefinedEqual \Expectation[F(x_k)] - F^*$.
  Applying \cref{th:UniversalFastSgd-GeneralGuarantee},
  dropping the nonnegative $\beta_{f, \bar{f}, \bar{g}}(\cdot, \cdot)$ terms
  and bounding $\Variance_{\hat{g}}(\cdot) \leq \sigma^2$, we obtain,
  for an arbitrary constant $\bar{M} > c_2 L_f$,
  \begin{align*}
    F_k
    &\leq
    \frac{1}{A_k} \Bigl(
      c_4 \bar{M} D^2
      +
      \frac{2 c_1 \sigma^2}{\bar{M} - c_2 L_f}
      \sum_{i = 1}^k a_i^2
      +
      c_3 \delta_f \sum_{i = 1}^k A_i
    \Bigr)
    \\
    &=
    \frac{4}{k (k + 1)}
    \Bigl(
      c_4 \bar{M} D^2
      +
      \frac{c_1 k (k + 1) (2 k + 1) \sigma^2}{12 (\bar{M} - c_2 L_f)}
      +
      \frac{c_3}{12} k (k + 1) (k + 2) \delta_f
    \Bigr)
    \\
    &=
    \frac{4 c_4 \bar{M} D^2}{k (k + 1)}
    +
    \frac{c_1 (2 k + 1) \sigma^2}{3 (\bar{M} - c_2 L_f)}
    +
    \delta_k,
  \end{align*}
  where $\delta_k \DefinedEqual \frac{c_3}{3} (k + 2) \delta_f$.
  We now choose $\bar{M} > c_2 L_f$ which minimizes the right-hand side.
  This is
  $
    \bar{M}
    =
    c_2 L_f
    +
    \frac{\sigma}{2 D} \sqrt{\frac{c_1}{3 c_4} k (k + 1) (2 k + 1)}
  $,
  for which we get
  \begin{align*}
    F_k
    &\leq
    \frac{4 c_4 D^2}{k (k + 1)}
    \biggl(
      c_2 L_f
      +
      \frac{\sigma}{2 D} \sqrt{\frac{c_1}{3 c_4} k (k + 1) (2 k + 1)} \,
    \biggr)
    +
    \frac{
      c_1 (2 k + 1) \sigma^2
    }{
      3
      \frac{\sigma}{2 D} \sqrt{\frac{c_1}{3 c_4} k (k + 1) (2 k + 1)}
    }
    +
    \delta_k
    \\
    &=
    \frac{4 c_2 c_4 L_f D^2}{k (k + 1)}
    +
    4 \sigma D \sqrt{\frac{c_1 c_4 (2 k + 1)}{3 k (k + 1)}}
    +
    \delta_k
    \leq
    \frac{4 c_2 c_4 L_f D^2}{k (k + 1)}
    +
    4 \sigma D \sqrt{\frac{2 c_1 c_4}{3 k}}
    +
    \delta_k.
    \qedhere
  \end{align*}
\end{proof}
