# Supplementary material for: Universality of AdaGrad Stepsizes for Stochastic Optimization: Inexact Oracle, Acceleration and Variance Reduction
Source: arXiv:2406.06398 source file (2024-06-10)
Supplement: Supplementary file 2 [file UniversalSgd.tex]

\subsection{Universal SGD}

\begin{lemma}[Stochastic Gradient Step]
  \label{th:StochasticGradientStep}
  Consider problem~\eqref{eq:Problem} under \cref{as:ApproximateSmoothness}.
  Let $\hat{g}$ be an unbiased oracle for $\bar{g}$.
  Let $x \in \EffectiveDomain \psi$ be a point, $M \geq 0$ be a coefficient,
  $\hat{g}_x \EqualRandom \hat{g}(x)$, and let
  \[
    \hat{x}_+ = \ProximalMap_{\psi}(x, \hat{g}_x, M).
  \]
  Denote
  $
    \hat{\Delta}(M)
    \DefinedEqual
    \beta_{f, \bar{f}, \bar{g}}(x, \hat{x}_+)
    +
    \InnerProduct{\bar{g}(x) - \hat{g}_x}{\hat{x}_+ - x}
    -
    \frac{M}{2} \Norm{\hat{x}_+ - x}^2
  $.
  Then,
  \[
    \Expectation\Bigl[
      F(\hat{x}_+) - F^* + \frac{M}{2} \Norm{\hat{x}_+ - x^*}^2
    \Bigr]
    +
    \beta_{f, \bar{f}, \bar{g}}(x, x^*)
    \leq
    \frac{M}{2} \Norm{x - x^*}^2
    +
    \Expectation[\hat{\Delta}(M)].
  \]
  If further \cref{as:BoundedFeasibleSet} is satisfied,
  and $\hat{M}_+ \geq M$ is a random coefficient
  (possibly dependent on~$\hat{g}_x$), then, we also have
  \[
    \Expectation\Bigl[
      F(\hat{x}_+) - F^* + \frac{\hat{M}_+}{2} \Norm{\hat{x}_+ - x^*}^2
    \Bigr]
    +
    \beta_{f, \bar{f}, \bar{g}}(x, x^*)
    \leq
    \frac{M}{2} \Norm{x - x^*}^2
    +
    \Expectation\bigl[ \hat{\Delta}(\hat{M}_+) + (\hat{M}_+ - M) D^2 \bigr].
  \]
\end{lemma}

\begin{proof}
  From \cref{th:OptimalityConditionForProximalStep}, it follows that
  \begin{multline*}
    \bar{f}(x) + \InnerProduct{\hat{g}_x}{\hat{x}_+ - x} + \psi(\hat{x}_+)
    +
    \frac{M}{2} \Norm{\hat{x}_+ - x^*}^2
    +
    \frac{M}{2} \Norm{\hat{x}_+ - x}^2
    \\
    \leq
    \bar{f}(x) + \InnerProduct{\hat{g}_x}{x^* - x} + \psi(x^*)
    +
    \frac{M}{2} \Norm{x - x^*}^2.
  \end{multline*}
  Passing to expectations and rewriting
  \[
    \Expectation[\bar{f}(x) + \InnerProduct{\hat{g}_x}{x^* - x} + \psi(x^*)]
    =
    \bar{f}(x) + \InnerProduct{\bar{g}(x)}{x^* - x} + \psi(x^*)
    =
    F(x^*) - \beta_{f, \bar{f}, \bar{g}}(x, x^*),
  \]
  and
  \begin{align*}
    \bar{f}(x) + \InnerProduct{\hat{g}_x}{\hat{x}_+ - x} + \psi(\hat{x}_+)
    &=
    F(\hat{x}_+)
    -
    [f(\hat{x}_+) - \bar{f}(x) - \InnerProduct{\hat{g}_x}{\hat{x}_+ - x}]
    \\
    &=
    F(\hat{x}_+)
    -
    [
      \beta_{f, \bar{f}, \bar{g}}(x, \hat{x}_+)
      +
      \InnerProduct{\bar{g}(x) - \hat{g}_x}{\hat{x}_+ - x}
    ],
  \end{align*}
  we obtain the first of the claimed inequalities.

  To prove the second one, we simply add to both sides of the already proved
  first inequality the expected value of
  \begin{multline*}
    \frac{\hat{M}_+ - M}{2} \Norm{\hat{x}_+ - x^*}^2
    +
    \hat{\Delta}(M) - \hat{\Delta}(\hat{M}_+)
    =
    \frac{\hat{M}_+ - M}{2}
    \bigl( \Norm{\hat{x}_+ - x^*}^2 + \Norm{\hat{x}_+ - x}^2 \bigr)
  \end{multline*}
  and then bound $\Norm{\hat{x}_+ - x^*} \leq D$, $\Norm{\hat{x}_+ - x} \leq D$
  using our \cref{as:BoundedFeasibleSet} and the fact that
  $x, \hat{x}_+, x^* \in \EffectiveDomain \psi$.
\end{proof}

\begin{lemma}[Universal Stochastic Gradient Step]
  \label{th:UniversalGradientStep}
  Consider problem~\eqref{eq:Problem} under
  \cref{as:BoundedFeasibleSet,as:ApproximateSmoothness}.
  Let $\hat{g}$ be an unbiased oracle for~$\bar{g}$.
  Further, let $x \in \EffectiveDomain \psi$ be a point,
  $M \geq 0$ be a coefficient, $\hat{g}_x \EqualRandom \hat{g}(x)$, and let
  \[
    \hat{x}_+ = \ProximalMap_{\psi}(x, \hat{g}_x, M),
    \quad
    \hat{g}_{x_+} \EqualRandom \hat{g}(\hat{x}_+),
    \quad
    \hat{M}_+ = M_+(M, D^2, x, \hat{x}_+, \hat{g}_x, \hat{g}_{x_+}).
  \]
  Then, for any $\bar{M} > c_2 L_f$, it holds that
  \begin{multline*}
    \Expectation\Bigl[
      F(\hat{x}_+) - F^*
      +
      \frac{\hat{M}_+}{2} \Norm{\hat{x}_+ - x^*}^2
      +
      \beta_{f, \bar{f}, \bar{g}}(\hat{x}_+, x)
    \Bigr]
    +
    \beta_{f, \bar{f}, \bar{g}}(x, x^*)
    \\
    \leq
    \frac{M}{2} \Norm{x - x^*}^2
    +
    \frac{c_1}{\bar{M} - c_2 L_f}
    \Expectation[\Variance_{\hat{g}}(\hat{x}_+) + \Variance_{\hat{g}}(x)]
    +
    c_3 \delta_f
    +
    c_4 \Expectation\bigl\{
      \PositivePart{\min\Set{\hat{M}_+, \bar{M}} - M} D^2
    \bigr\}.
  \end{multline*}
\end{lemma}

\begin{proof}
  According to \cref{th:StochasticGradientStep},
  \[
    \Expectation\Bigl[
      F(\hat{x}_+) - F^* + \frac{\hat{M}_+}{2} \Norm{\hat{x}_+ - x^*}^2
    \Bigr]
    +
    \beta_{f, \bar{f}, \bar{g}}(x, x^*)
    \leq
    \frac{M}{2} \Norm{x - x^*}^2
    +
    \Expectation\bigl[ \hat{\Delta}(\hat{M}_+) + (\hat{M}_+ - M) D^2 \bigr],
  \]
  where
  $
    \hat{\Delta}(\hat{M}_+)
    \DefinedEqual
    \beta_{f, \bar{f}, \bar{g}}(x, \hat{x}_+)
    +
    \InnerProduct{\bar{g}(x) - \hat{g}_x}{\hat{x}_+ - x}
    -
    \frac{\hat{M}_+}{2} \Norm{\hat{x}_+ - x}^2
  $.
  At the same time, according to the main
  requirement~\eqref{eq:RequirementOnStepsizeUpdateRule} on the stepsize update
  rule, for any $\bar{M} > c_2 L_f$,
  \begin{multline*}
    \Expectation\bigl[
      \hat{\Delta}(\hat{M}_+)
      +
      (\hat{M}_+ - M) D^2
      +
      \beta_{f, \bar{f}, \bar{g}}(\hat{x}_+, x)
    \bigr]
    \\
    \leq
    \frac{c_1}{\bar{M} - c_2 L_f}
    \Expectation[\Variance_{\hat{g}}(\hat{x}_+) + \Variance_{\hat{g}}(x)]
    +
    c_3 \delta{_f}
    +
    c_4 \Expectation\bigl\{
      \PositivePart{\min\Set{\hat{M}_+, \bar{M}} - M} D^2
    \bigr\}.
  \end{multline*}
  Combining the two displays, we get the claim.
\end{proof}

\begin{lemma}[Universal SGD: General Guarantee]
  \label{th:UniversalSgd-General}
  Consider problem~\eqref{eq:Problem} under
  \cref{as:BoundedFeasibleSet,as:ApproximateSmoothness}.
  Let $\hat{g}$ be an unbiased oracle for~$\bar{g}$.
  Further, let $x \in \EffectiveDomain \psi$ be a point,
  $M \geq 0$ be a coefficient, $N \geq 1$ be an integer, and let
  \[
    (\bar{x}_N, x_N, M_N)
    \EqualRandom
    \UniversalSgd_{\hat{g}, \psi}(x_0, M_0, N; D),
  \]
  as defined by \cref{alg:UniversalSgd},
  and let $x_0, \ldots, x_N$ be the corresponding points generated inside the
  algorithm.
  Then, for any $\bar{M} > c_2 L_f$, it holds that
  \begin{multline*}
    \Expectation\Bigl[
      N [F(\bar{x}_N) - F^*]
      +
      \frac{M_N}{2} \Norm{x_N - x^*}^2
      +
      \sum_{k = 0}^{N - 1} [
        \beta_{f, \bar{f}, \bar{g}}(x_{k + 1}, x_k)
        +
        \beta_{f, \bar{f}, \bar{g}}(x_k, x^*)
      ]
    \Bigr]
    \\
    \leq
    \frac{M_0}{2} \Norm{x_0 - x^*}^2
    +
    \frac{c_1}{\bar{M} - c_2 L_f}
    \sum_{k = 0}^{N - 1}
    \Expectation[\Variance_{\hat{g}}(x_{k + 1}) + \Variance_{\hat{g}}(x_k)]
    +
    c_3 N \delta_f
    \\
    +
    c_4 \Expectation\bigl\{
      \PositivePart{\min\Set{M_N, \bar{M}} - M_0} D^2
    \bigr\}.
  \end{multline*}
\end{lemma}

\begin{proof}
  Each iteration~$k$ of the algorithm, when conditioned on~$x_k$, follows the
  construction from \cref{th:UniversalGradientStep}
  (with $x = x_k$, $\hat{g}_x = g_k$, $M = M_k$, $\hat{x}_+ = x_{k + 1}$,
    $\hat{g}_{x_+} = g_{k + 1}$, $\hat{M}_+ = M_{k + 1}$).
  Hence, we can write, after passing to full expectations, that,
  for each $k = 0, \ldots, N - 1$,
  \begin{multline*}
    \Expectation\Bigl[
      F(x_{k + 1}) - F^*
      +
      \frac{M_{k + 1}}{2} \Norm{x_{k + 1} - x^*}^2
      +
      \beta_{f, \bar{f}, \bar{g}}(x_{k + 1}, x_k)
      +
      \beta_{f, \bar{f}, \bar{g}}(x_k, x^*)
    \Bigr]
    \\
    \leq
    \Expectation\Bigl[
      \frac{M_k}{2} \Norm{x_k - x^*}^2
      +
      \frac{c_1}{\bar{M} - c_2 L_f}
      [\Variance_{\hat{g}}(x_{k + 1}) + \Variance_{\hat{g}}(x_k)]
      +
      c_4 \PositivePart{\min\Set{M_{k + 1}, \bar{M}} - M_k} D^2
    \Bigr]
    +
    c_3 \delta_f,
  \end{multline*}
  where $\bar{M} > 2 L_f$ is an arbitrary constant.
  Telescoping the above inequalities
  (using \cref{th:TelescopingDifferencesWithMin}) and then
  bounding $N [F(\bar{x}_N) - F^*] \leq \sum_{k = 1}^N [F(x_k) - F^*]$
  (using the convexity of~$F$ and our choice of
    $\bar{x}_N = \frac{1}{N} \sum_{k = 1}^N x_k$), we get the claim.
\end{proof}

\thComplexityOfUniversalSgd*

\begin{proof}
  \label{th:UniversalSgd:Proof}
  Applying \cref{th:UniversalSgd-General},
  substituting our choice of $M_0 = 0$,
  estimating $\Variance_{\hat{g}}(\cdot) \leq \sigma^2$ and dropping the
  nonnegative $\beta_{f, \bar{f}, \bar{g}}(\cdot, \cdot)$ terms, we obtain
  \[
    \Expectation[F(\bar{x}_N)] - F^*
    \leq
    \frac{1}{N} \Bigl(
      c_4 \bar{M} D^2
      +
      \frac{2 c_1 \sigma^2 N}{\bar{M} - c_2 L_f}
      +
      c_3 N \delta_f
    \Bigr)
    =
    \frac{c_4 \bar{M} D^2}{N}
    +
    \frac{2 c_1 \sigma^2}{\bar{M} - c_2 L_f}
    +
    c_3 \delta_f,
  \]
  where $\bar{M} > 2 L_f$ is an arbitrary constant.
  The optimal $\bar{M}$ which minimizes the right-hand side is
  $\bar{M} = c_2 L_f + \frac{\sigma}{D} \sqrt{\frac{2 c_1}{c_4} N}$.
  Substituting this choice into the above display, we get
  \begin{align*}
    \Expectation[F(\bar{x}_N)] - F^*
    &\leq
    \frac{c_4 D^2}{N} \Bigl(
      c_2 L_f + \frac{\sigma}{D} \sqrt{\frac{2 c_1}{c_4} N}
    \Bigr)
    +
    \frac{2 c_1 \sigma^2}{\frac{\sigma}{D} \sqrt{\frac{2 c_1}{c_4} N}}
    +
    c_3 \delta_f
    \\
    &=
    \frac{c_2 c_4 L_f D^2}{N}
    +
    2 \sigma D \sqrt{\frac{2 c_1 c_4}{N}}
    +
    c_3 \delta_f.
    \qedhere
  \end{align*}
\end{proof}
